# Supplementary material for: PO-EMO: Conceptualization, Annotation, and Modeling of Aesthetic Emotions in German and English Poetry
Source: arXiv:2003.07723 source file (2021-06-23)
Supplement: Supplementary file 1 [file 7_appendix.tex]

\newpage
\section*{Appendix / Guidelines}

\subsection*{INSTRUCTIONS FOR ANNOTATING}
\begin{enumerate}
\item The annotation should reflect your current feelings while reading the poem.
\item Label your emotions after reading each individual line (not sentence!).
\item Read the entire stanza before annotating each line.
\item Use as few emotions as possible!
\item Choose at least one label per line.
\item You should not use more than two labels per line.
\item Choose the emotion most dominant while reading the stanza.
\item Choose another emotion if necessary.
\item Only change the dominant emotion within a stanza, if unavoidable.
\item If you change the non-dominant emotion within a stanza, remember to keep labelling the
dominant emotion additionally to the new emotion.
\item Notice that nostalgia always has to be used with an additonal label: beauty/joy or sadness
\end{enumerate}

\subsection*{LABEL SET / EXAMPLES}

\subsubsection*{Annoyance} (annoys me / angers me / felt frustrated) \\
Choose this label if you feel annoyed, frustrated or even angry while reading the line/stanza. \\
Example 1\\
\begin{table}[ht!]
\centering
\begin{scriptsize}
\begin{tabular}{lll}
In every cry of every Man, &[Sadness] & \textcolor{red}{[Annoyance]}\\
In every Infants cry of fear, &[Sadness] & \textcolor{red}{[Annoyance]}\\
In every voice: in every ban, &[Sadness] & \textcolor{red}{[Annoyance]}\\
The mind-forg'd manacles I hear &[Sadness] & \textcolor{red}{[Annoyance]}\\
How the Chimney-sweepers cry &[Sadness] & \textcolor{red}{[Annoyance]}\\
Every blackning Church appalls, &[Sadness] & \textcolor{red}{[Annoyance]}\\
And the hapless Soldiers sigh &[Sadness] & \textcolor{red}{[Annoyance]}\\
Runs in blood down Palace walls &[Sadness] & \textcolor{red}{[Annoyance]}\\
But most thro' midnight streets I hear &[Sadness] & \textcolor{red}{[Annoyance]}\\
How the youthful Harlots curse &[Sadness] & \textcolor{red}{[Annoyance]}\\
Blasts the new-born Infants tear &[Sadness] & \textcolor{red}{[Annoyance]}\\
And blights with plagues the Marriage hearse &[Sadness] & \textcolor{red}{[Annoyance]}\\
\end{tabular}
\end{scriptsize}
\end{table}
\paragraph{Awe/Sublime} (found it overwhelming / sense of greatness) \\
Choose this label if you feel overwhelmed by the line/stanza, i.e. if you get the impression of facing
something sublime or if the line / stanza inspires you with awe (such emotions are often associated with
subjects like god, death, life, truth etc.).
\paragraph{Beauty/Joy} (found it beautiful/ pleasing/ makes me happy/ joyful) \\
Choose this label if you feel pleasure from reading the line/stanza (if the line/stanza puts you into a
happy/joyful mood).
\paragraph{Humor} (found it funny / amusing) \\
Choose this label if you feel amused by the line/stanza (if the line/stanza even makes you laugh).
\paragraph{Nostalgia} (makes me nostalgic) \\
Use this label only in addition with another label: + beauty/joy or + sadness!
Choose this label if the line/stanza evokes feelings of nostalgia. Nostalgia is defined as a sentimental
longing for things, persons or situations in the past. It’s possible to feel nostalgic about things you haven’t
experienced by your own. Notice to annotate your feeling of nostalgia together with +beauty/joy (if
positive feelings) or +sadness (if negative feelings).
\paragraph{Sadness} (makes me sad / touches me) \\
Choose this label if the line/stanza makes you feel sad.
\paragraph{Suspense} (found it gripping / sparked my interest)
Choose this label if the line/stanza keeps you in suspense (if the line/stanza excites you or triggers your
curiosity)
\paragraph{Uneasiness} (found it ugly / unsettling / disturbing / frightening / distasteful) \\
Choose this label, if you feel discomfort about the line/stanza (if the line/stanza feels distasteful/ugly,
unsettling/disturbing or frightens you).
\paragraph{Vitality} (found it invigorating / spurs me on / inspires me) \\
Choose this label if the line/stanza has an inciting, encouraging effect. (If the line/stanza conveys a feeling of movement, energy and vitality which it can pass over to you)

\subsection*{Gold Standard}
The following examples serve as an orientation for the annotators. The exemplary emotion is highlighted.
When in doubt, then gold standard!

\paragraph{Annoyance} (annoys me, angers me, felt frustrated) \\

\paragraph{Awe/Sublime} (found it overwhelming/sense of greatness)\\
Example 1
From harmony, from Heav'nly harmony \textcolor{red}{[Awe / Sublime]} [Beauty/Joy]
This universal frame began. [Awe / Sublime] [Beauty/Joy]
When Nature underneath a heap [Awe / Sublime] [Beauty/Joy]
Of jarring atoms lay, [Awe / Sublime] [Beauty/Joy]
And could not heave her head, [Awe / Sublime] [Beauty/Joy]
The tuneful voice was heard from high, [Awe / Sublime] [Beauty/Joy]
Arise ye more than dead. [Awe / Sublime] [Beauty/Joy]
Then cold, and hot, and moist, and dry, [Awe / Sublime] [Beauty/Joy]
In order to their stations leap, [Awe / Sublime] [Beauty/Joy]
And music's pow'r obey. [Awe / Sublime] [Beauty/Joy]
From harmony, from Heav'nly harmony [Awe / Sublime] [Beauty/Joy]
This universal frame began: [Awe / Sublime] [Beauty/Joy]
From harmony to harmony [Awe / Sublime] [Beauty/Joy]
Through all the compass of the notes it ran, [Awe / Sublime] [Beauty/Joy]
The diapason closing full in man. [Awe / Sublime] [Beauty/Joy]
Example 2
The moving waters at their priestlike task [Awe / Sublime]
Of pure ablution round earth's human shores, [Awe / Sublime]
4
Or gazing on the new soft-fallen mask [Awe / Sublime]
Of snow upon the mountains and the moors— [Awe / Sublime]
• Beauty/Joy (found it beautiful/ pleasing/ makes me happy/ joyful)
Example 1
i carry your heart with me(i carry it in [Beauty/Joy]
my heart)i am never without it(anywhere [Beauty/Joy]
i go you go, my dear; and whatever is done [Beauty/Joy]
by only me is your doing, my darling) [Beauty/Joy]
i fear [Beauty/Joy]
no fate(for you are my fate, my sweet)i want [Beauty/Joy]
no world(for beautiful you are my world, my true) [Beauty/Joy]
and it's you are whatever a moon has always meant [Beauty/Joy]
and whatever a sun will always sing is you [Beauty/Joy]
Example 2
How do I love thee? Let me count the ways, [Beauty/Joy]
I love thee to the depth and breadth and height [Beauty/Joy]
My soul can reach, when feeling out of sight [Beauty/Joy]
For the ends of being and ideal grace. [Beauty/Joy]
I love thee to the level of every day's [Beauty/Joy]
Most quiet need, by sun and candle-light, [Beauty/Joy]
I love thee freely, as men strive for right. [Beauty/Joy]
I love thee purely, as they turn from praise, [Beauty/Joy]
I love thee with the passion put to use [Beauty/Joy]
In my old griefs, and with my childhood's faith. [Beauty/Joy]
I love thee with a love I seemed to lose [Beauty/Joy] [Awe/Sublime]
With my lost saints. I love thee with the breath, [Beauty/Joy] [Awe/Sublime]
Smiles, tears, of all my life; and, if God choose, [Beauty/Joy] [Awe/Sublime]
I shall but love thee better after death. [Beauty/Joy] [Awe/Sublime]
• Humor (found it funny/ amusing)
Example 1
I'm Nobody! Who are you? [Humor]
Are you - Nobody - too? [Humor]
Then there's a pair of us! [Humor]
Dont tell! they'd advertise - you know! [Humor]
How dreary - to be - Somebody! [Humor]
How public - like a Frog - [Humor]
To tell one's name - the livelong June - [Humor]
To an admiring Bog! [Humor]
• Nostalgia (makes me nostalgic)
5
Example 1
John Anderson my jo, John, [Nostalgia] [Sadness]
When we were first acquent, [Nostalgia] [Sadness]
Your locks were like the raven, [Nostalgia] [Sadness]
Your bonie brow was brent; [Nostalgia] [Sadness]
But now your brow is beld, John, [Nostalgia] [Sadness]
Your locks are like the snaw, [Nostalgia] [Sadness]
but blessings on your frosty pow, [Nostalgia] [Sadness]
John Anderson, my jo! [Nostalgia] [Sadness]
Example 2
Thou'll break my heart, thou bonnie bird, [Sadness]
That sings upon the bough; [Sadness]
Thou minds me o' the happy days [Nostalgia] [Sadness]
When my fause luve was true. [Nostalgia] [Sadness]
• Sadness (makes me sad/touches me)
Example 1
I felt a Funeral, in my Brain, [Sadness]
And Mourners to and fro [Sadness]
Kept treading - treading - till it seemed [Sadness]
That Sense was breaking through - [Sadness]
Example 2
My spirit is too weak—mortality [Sadness]
Weighs heavily on me like unwilling sleep, [Sadness]
And each imagined pinnacle and steep [Sadness]
Of godlike hardship tells me I must die [Sadness]
Like a sick eagle looking at the sky. [Sadness]
• Suspense (found it gripping/sparked my interest)
Example 1
The Second Coming! Hardly are those words out [Uneasiness] [Suspense]
When a vast image out of Spiritus Mundi [Uneasiness] [Suspense]
Troubles my sight: somewhere in sands of the desert [Uneasiness] [Suspense]
A shape with lion body and the head of a man, [Uneasiness] [Suspense]
A gaze blank and pitiless as the sun, [Uneasiness] [Suspense]
Is moving its slow thighs, while all about it [Uneasiness] [Suspense]
Reel shadows of the indignant desert birds. [Uneasiness] [Suspense]
• Uneasiness (found it ugly/unsettling/disturbing/frightening/distasteful)
Example 1
6
To wait in heavy harness [Uneasiness]
On fluttered folk and wild - [Uneasiness]
Your new-caught sullen peoples, [Uneasiness]
Half devil and half child. [Uneasiness]
Example 2
They are rattling breakfast plates in basement kitchens, [Uneasiness]
And along the trampled edges of the street [Uneasiness]
I am aware of the damp souls of housemaids [Uneasiness]
Sprouting despondently at area gates. [Uneasiness]
• Vitality (found it invigorating/spurs me on/inspires me)
Example 1
Be fair or foul or rain or shine [Vitality]
The joys I have possessed, in spite of fate, are mine. [Vitality]
Not Heaven itself upon the past has power, [Vitality]
But what has been, has been, and I have had my hour. [Vitality]
Example 2
Break, break, break, [Vitality]
On thy cold gray stones, O Sea! [Vitality]
And I would that my tongue could utter [Vitality]
The thoughts that arise in me. [Vitality]
